# Supplementary material for: Smart Bird: Learnable Sparse Attention for Efficient and Effective Transformer
Source: arXiv:2108.09193 source file (2021-09-02)
Supplement: Supplementary file 1 [file supplement.tex]

\section*{Supplementary Materials}

\subsection*{Experimental Environment}

We conduct experiments on a Linux machine with Ubuntu 16.04 operating system.
The codes are written in Python 3.7 using the Keras library 2.2.4 with Tensorflow 1.12 backend.
The GPU type is GTX 1080 ti with a memory of 12GB.
The CPU type is Xeon(R) CPU E5-2620 v4 \@ 2.10GHz.
All codes are run on a single GPU with a single process.

\subsection*{Preprocessing}

In our experiments, we use the NLTK tool to preprocess the documents.
We use the word\_tokenize and sent\_tokenize function respectively for word and sentence tokenization.
Since the total vocabulary is too large for our GPU memory, we filter the words with frequencies less than 3, 5, and 10 respectively on the Amazon, IMDB and MIND datasets.
The word embeddings of out-of-vocabulary words are filled with random vectors that have the same mean and co-variation values as other words. 

\subsection*{Hyperparameter Settings}

The detailed hyperparameter settings in this paper are listed in Table~\ref{hyper}.

\begin{table}[h]
\centering
%\resizebox{1.0\linewidth}{!}{
\begin{tabular}{|l|c|}
\hline
\multicolumn{1}{|c|}{\textbf{Hyperparameters}}& \textbf{Value} \\ \hline
word embedding dim.                     & 300            \\ 
\# self-attention heads                  & 8             \\
output dim. of each head               & 32            \\
\# layers               & 2            \\
dropout                                      & 0.2            \\
optimizer                                    & Adam           \\
learning rate                                & 1e-4           \\
batch size                                   & 64    \\     epoch                              & 2    \\     \hline
\end{tabular}
%}
\caption{Detailed hyperparameter settings.}\label{hyper}
\end{table}

\subsection*{Validation Performance}

The results of different methods on the validation set are shown in Table~\ref{table.performance2}.

\begin{table*}[!t]
\resizebox{0.98\textwidth}{!}{
\begin{tabular}{lcccccc}
\Xhline{1.5pt}
\multicolumn{1}{c}{\multirow{2}{*}{Methods}} & \multicolumn{2}{c}{Amazon}      & \multicolumn{2}{c}{IMDB} & \multicolumn{2}{c}{MIND} \\ \cline{2-7} 
\multicolumn{1}{c}{}                         & Accuracy       & Macro-F        & Accuracy    & Macro-F    & Accuracy    & Macro-F    \\ \hline
Transformer                                  & 65.31$\pm$0.35 & 42.28$\pm$0.36 & 52.06$\pm$0.45       & 42.81$\pm$0.46     & 81.11$\pm$0.24       & 60.05$\pm$0.25      \\
Longformer                                   & 65.40$\pm$0.42 & 42.51$\pm$0.44 & 52.29$\pm$0.39       & 43.56$\pm$0.44     & 81.37$\pm$0.27       & 62.75$\pm$0.30      \\
BigBird                                     & 66.12$\pm$0.54 & 42.79$\pm$0.50 & 52.96$\pm$0.48       & 43.75$\pm$0.49     & 81.94$\pm$0.30       & 63.55$\pm$0.28      \\
Hierarchical Transformer                     & 66.40$\pm$0.43 & 42.70$\pm$0.39 & 53.11$\pm$0.43       & 43.94$\pm$0.40     & 81.95$\pm$0.22       & 63.67$\pm$0.25      \\ \hline
Hi-Transformer*                               & 67.33$\pm$0.28 & 43.74$\pm$0.34 & 53.69$\pm$0.51       & 44.62$\pm$0.50     & 82.47$\pm$0.24       & 64.21$\pm$0.19      \\  \Xhline{1.5pt}
\end{tabular}
}
\caption{Performance of different methods on the validation sets.} \label{table.performance2} 
\end{table*}
